# Supplementary material for: DMTG: One-Shot Differentiable Multi-Task Grouping
Source: arXiv:2407.05082 source file (2024-07-06)
Supplement: Supplementary file 1 [file 6_appendix.tex]

%%%%%%%%%%%%%%%%%%%%%%%%%%%%%%%%%%%%%%%%%%%%%%%%%%%%%%%%%%%%%%%%%%%%%%%%%%%%%%%
%%%%%%%%%%%%%%%%%%%%%%%%%%%%%%%%%%%%%%%%%%%%%%%%%%%%%%%%%%%%%%%%%%%%%%%%%%%%%%%
% APPENDIX
%%%%%%%%%%%%%%%%%%%%%%%%%%%%%%%%%%%%%%%%%%%%%%%%%%%%%%%%%%%%%%%%%%%%%%%%%%%%%%%
%%%%%%%%%%%%%%%%%%%%%%%%%%%%%%%%%%%%%%%%%%%%%%%%%%%%%%%%%%%%%%%%%%%%%%%%%%%%%%%
\newpage
\appendix
\twocolumn
\section{Appendix}
\subsection{Datasets}
\noindent \textbf{CelebA} \cite{faceattribute2015} is a large-scale face dataset that contains more than $200,000$ images from roughly $10,000$ identities, each of which has annotated $40$ face attributes representing the tasks to predict. Samples of CelebA datasets are illustrated in Fig. \ref{img:celeba}. For the CelebA experiments, the $9$ tasks implemented in CelebA-$9$ \cite{tag2021} are \textit{5\_o\_Clock\_Shadow}, \textit{Black\_Hair}, \textit{Blond\_Hair}, \textit{Brown\_Hair}, \textit{Goatee}, \textit{Mustache}, \textit{No\_Beard}, \textit{Rosy\_Cheeks}, and \textit{Wearing\_Hat}. We also testify our method with CelebA-$40$ using all the 40 labeled attributes of the CelebA dataset. All images in the CelebA dataset are resized to $64\times64$ resolution.

\textbf{Taskonomy} \cite{taskonomy2018} is one of the largest  datasets with multi-task labels, covering 26 vision tasks from 2D to 3D. For the Taskonomy experiments, we use the official tiny train, validation, and test split with roughly $300,000$ images. The tasks used to learn the categorization are the same as those in \cite{hoa2020,tag2021,mtg2022}, which are \textit{semantic segmentation}, \textit{depth estimation}, \textit{surface normal}, \textit{keypoint detection}, and \textit{canny edge detection}, as shown in Figure \ref{img:taskonomy}. We also follow \cite{hoa2020,tag2021,mtg2022} to bilinearly downsample the Taskonomy images to $256\times 256$ before training and testing. 

\begin{figure}[t]
    \centering
    \includegraphics[width=0.88\columnwidth]{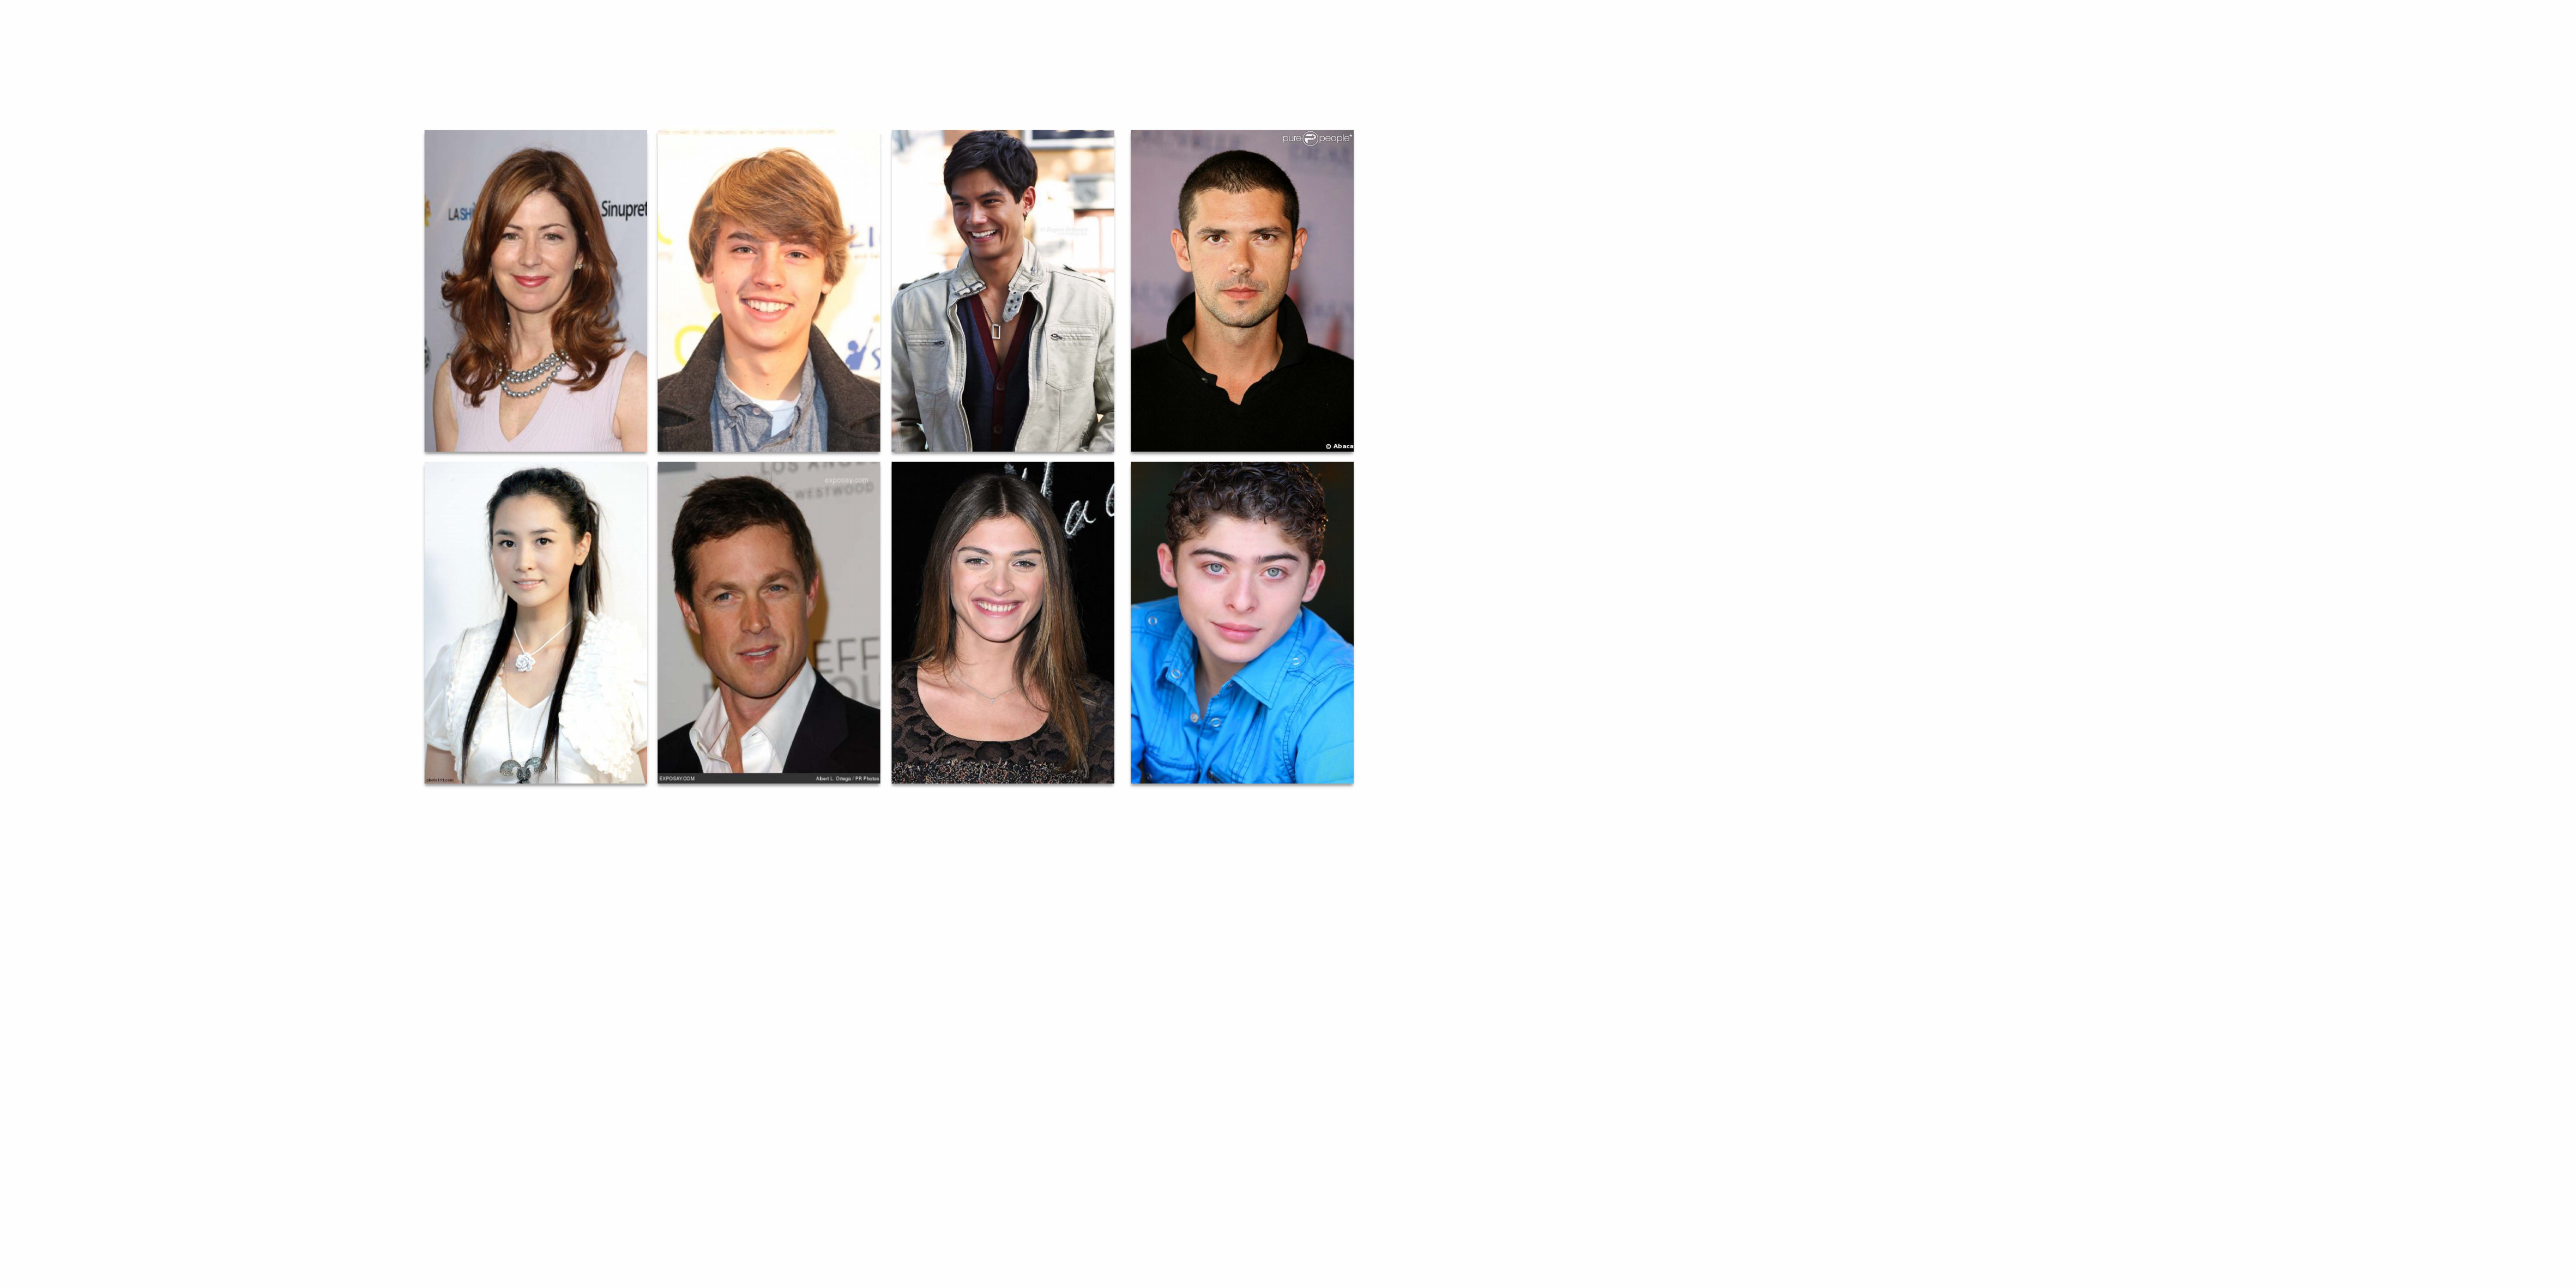}
    \caption{Illustration of the CelebA dataset.}
    \label{img:celeba}
\end{figure}

\begin{figure}[t]
    \centering
    \includegraphics[width=0.88\columnwidth]{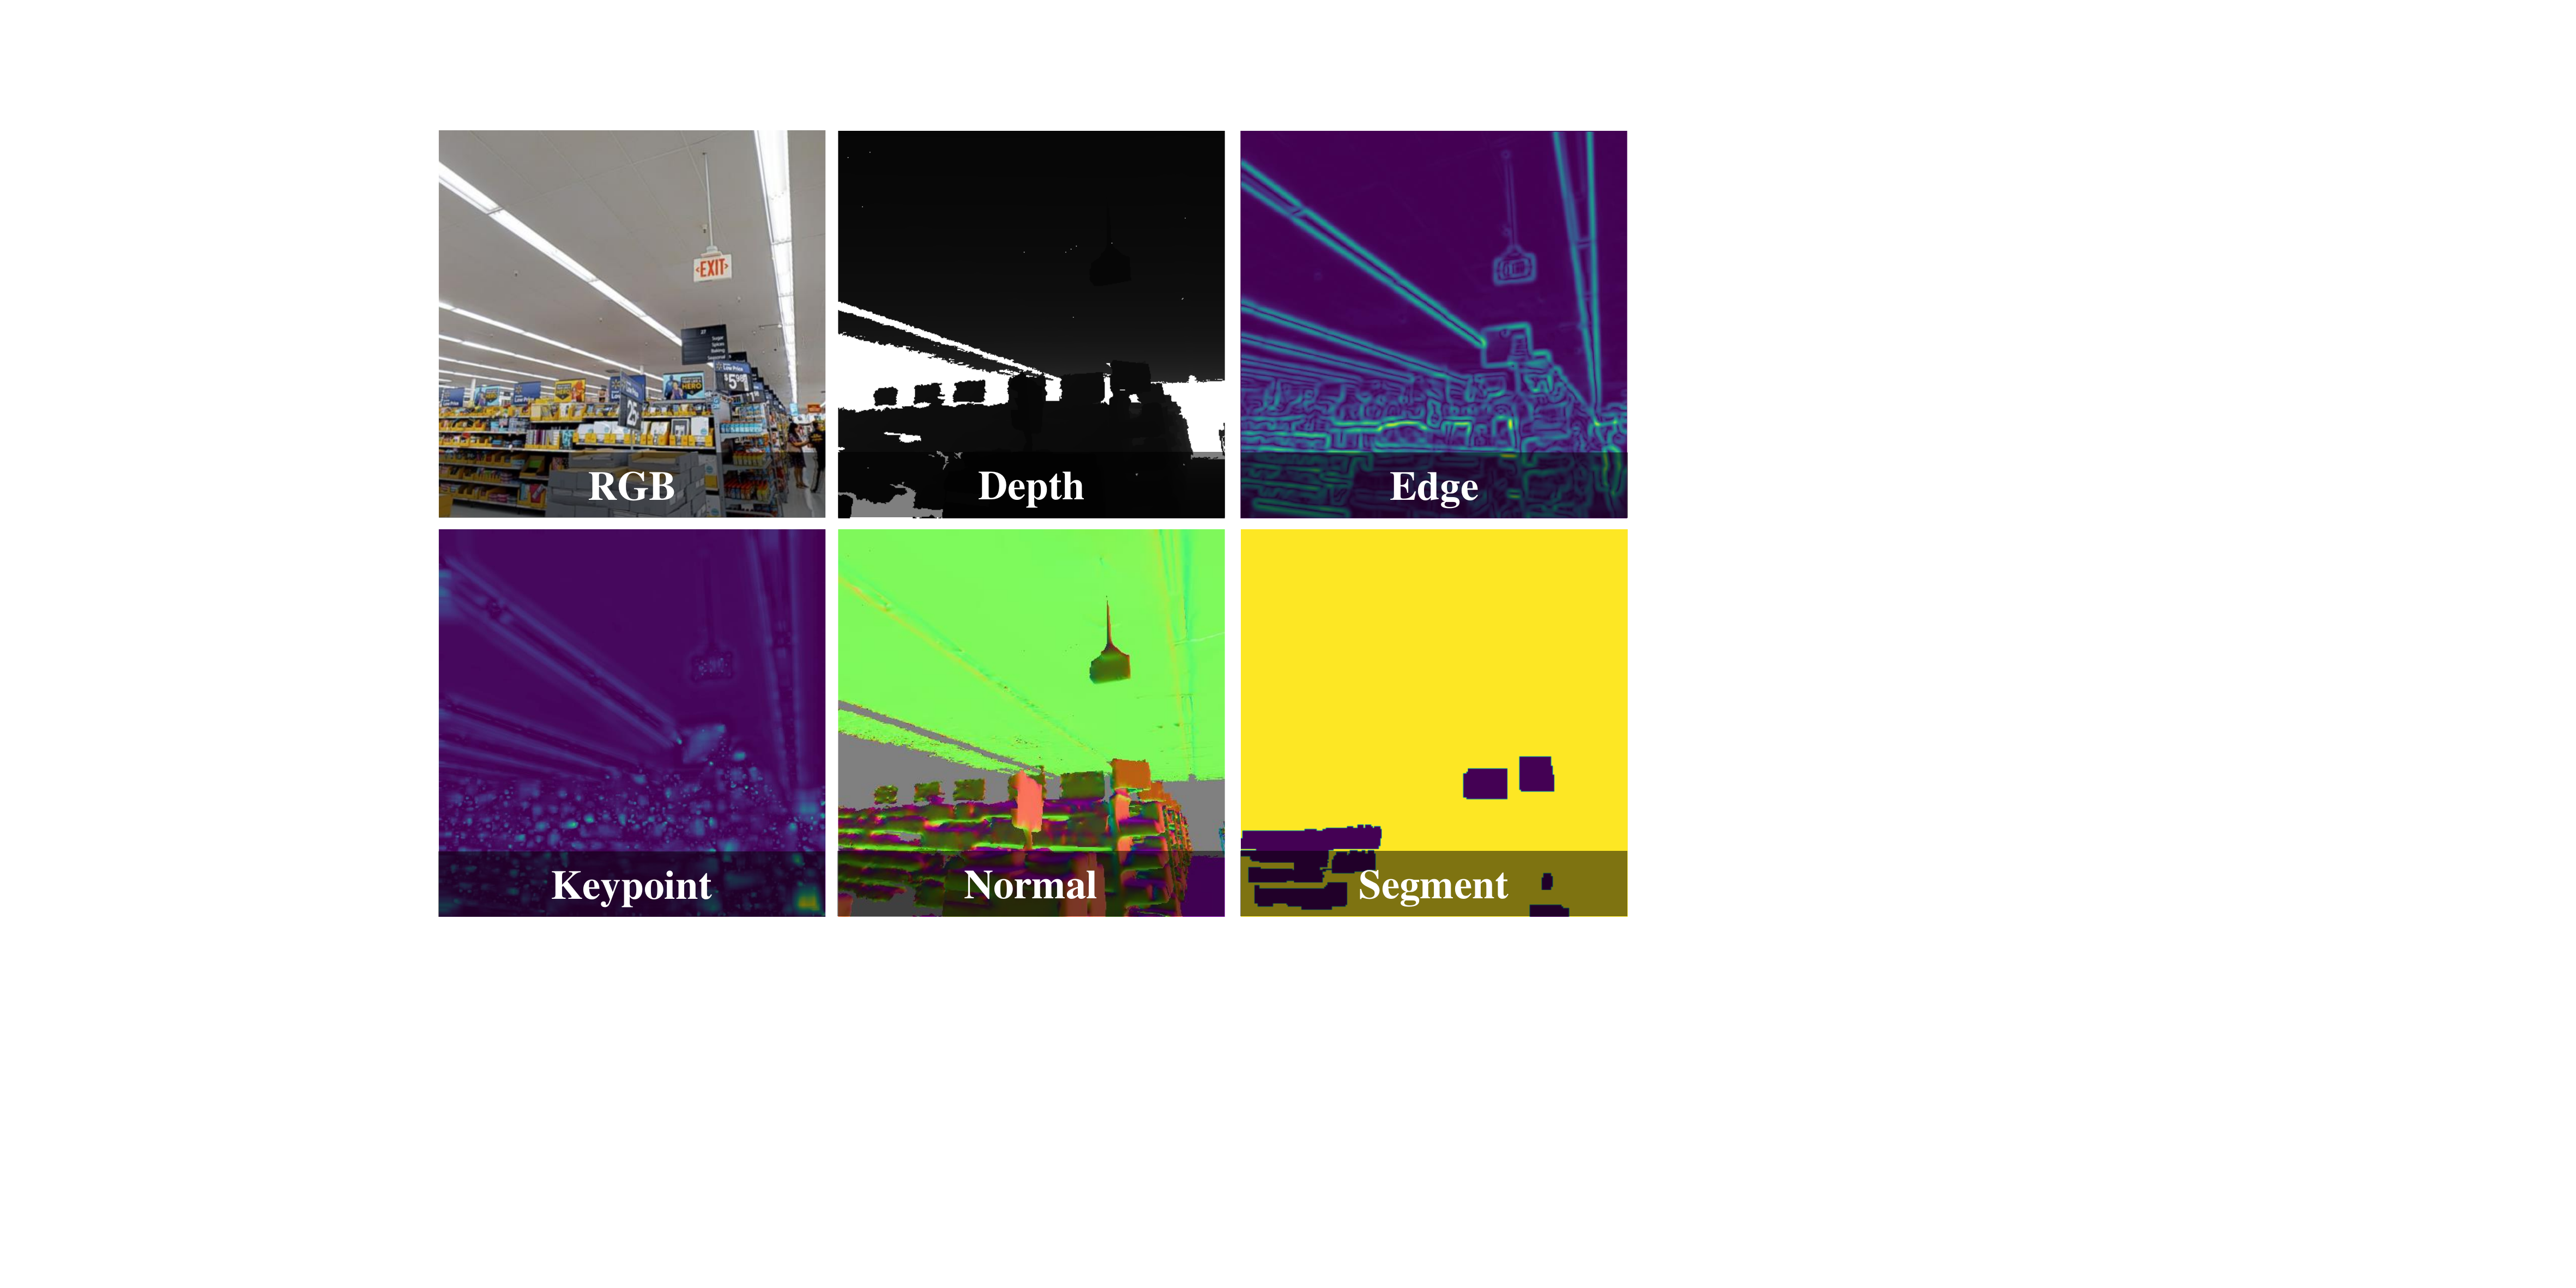}
    \caption{Illustration of the Taskonomy dataset.}
    \label{img:taskonomy}
\end{figure}

\subsection{Relative improvement to STL}
\label{subsec: relative to stl}
Figure \ref{stl radar} displays three radar plots concerning the improvement of grouping methods on each task relative to STL, for $K=3, 4, 5$. In these plots, our approach covers a significantly large area, showcasing substantial advantages over other methods. Whether compared to naive MTL or STL, the proposed method demonstrates remarkable improvements across all tasks. In conclusion, it proves to be more robust than current methods in grouping tasks and entails only $O(K)$ training complexity. This takes a step forward in grouping tasks, making it feasible to run in practical applications.

\begin{figure*}[t]
    \centering
    \includegraphics[width=0.85\textwidth]{image/taskonomy_radar_stl.pdf}
    \caption{Relative improvement of our method in terms of STL for each task on the Taskonomy dataset with 5 tasks over 3, 4, and 5 groups. The value of relative improvement lower than $-0.2$ has been truncated here.}
    \label{stl radar}
\end{figure*}

\begin{table*}[t]
\centering
\resizebox{0.99\textwidth}{!}{
    \begin{tabular}{l|l|ccccc}
    \hline
Method                   & Splits  & Depth estimation  & Surface normal    & Semantic segmentation & Keypoint detection & Canny edge detection \\ \hline
\multirow{3}{*}{HOA}     & group 1 & \checkmark          & \textcolor{red}{\checkmark} & \checkmark              & -                  & -                    \\
                         & group 2 & -                 & \checkmark          & -                     & \checkmark           & -                    \\
                         & group 3 & -                 & -                 & -                     & \textcolor{red}{\checkmark}  & \textcolor{red}{\checkmark}    \\ \hline
\multirow{3}{*}{TAG}     & group 1 & \textcolor{red}{\checkmark} &                   & \textcolor{red}{\checkmark}     & -                  & -                    \\
                         & group 2 & \checkmark          & \textcolor{red}{\checkmark} & -                     & -                  & -                    \\
                         & group 3 & -                 & -                 & -                     & \textcolor{red}{\checkmark}  & \textcolor{red}{\checkmark}    \\ \hline
\multirow{3}{*}{MTG-Net} & group 1 & \checkmark          & \textcolor{red}{\checkmark} & \textcolor{red}{\checkmark}     & \checkmark           & \checkmark             \\
                         & group 2 & \checkmark          & \checkmark          & -                     & \textcolor{red}{\checkmark}  & -                    \\
                         & group 3 & \textcolor{red}{\checkmark} & \checkmark          & -                     & -                  & \textcolor{red}{\checkmark}    \\ \hline
\multirow{3}{*}{Ours}    & group 1 & -                 & -                 & -                     & -                  & -                    \\
                         & group 2 & \textcolor{red}{\checkmark} & -                 & -                     & -                  & \textcolor{red}{\checkmark}    \\ 
                         & group 3 & -                 & \textcolor{red}{\checkmark} & \textcolor{red}{\checkmark}     & \textcolor{red}{\checkmark}  & -    \\ \hline                   
\end{tabular}}
\caption{task loss on taskonomy when K=3}
\label{}
\end{table*}

\begin{table*}[t]
\centering
\resizebox{0.99\textwidth}{!}{
    \begin{tabular}{l|l|ccccc}
    \hline
Method                   & Splits  & Depth estimation  & Surface normal    & Semantic segmentation & Keypoint detection & Canny edge detection \\ \hline
\multirow{4}{*}{HOA}     & group 1 & -                 & \checkmark          & -                     & \checkmark           & -                    \\
                         & group 2 & -                 & -                 & -                     & \textcolor{red}{\checkmark}  & \textcolor{red}{\checkmark}    \\
                         & group 3 & -                 & \textcolor{red}{\checkmark} & \textcolor{red}{\checkmark}     & -         & -           \\
                         & group 4 & \textcolor{red}{\checkmark} & \checkmark          & -                     & -         & -           \\ \hline
\multirow{4}{*}{TAG}     & group 1 & \checkmark          & -                 & \checkmark              & -                  & -                    \\
                         & group 2 & \textcolor{red}{\checkmark} & \checkmark          & -                     & -                  & -                    \\
                         & group 3 & -                 & -                 & -                     & \textcolor{red}{\checkmark}  & \textcolor{red}{\checkmark}    \\
                         & group 4 & \checkmark          & \textcolor{red}{\checkmark} & \textcolor{red}{\checkmark}     & -         & -           \\ \hline
\multirow{4}{*}{MTG-Net} & group 1 & \checkmark          & \textcolor{red}{\checkmark} & \textcolor{red}{\checkmark}     & \checkmark           & \checkmark             \\
                         & group 2 & \checkmark          & \checkmark          & -                     & \textcolor{red}{\checkmark}  & -                    \\
                         & group 3 & \textcolor{red}{\checkmark} & \checkmark          & -                     & -                  & \textcolor{red}{\checkmark}    \\
                         & group 4 & \checkmark          & \checkmark          & -                     & -                  & -                    \\ \hline
\multirow{4}{*}{Ours}    & group 1 & \textcolor{red}{\checkmark} & -                 & -                     & -                  & -    \\
                         & group 2 & -        & -                 & -                     & -                  & -           \\
                         & group 3 & -                 & \textcolor{red}{\checkmark} & \textcolor{red}{\checkmark}     & \textcolor{red}{\checkmark}  & \textcolor{red}{\checkmark}                    \\
                         & group 4 & -        & -                 & -                     & -                  & - \\ \hline                    
\end{tabular}}
    \caption{task loss on taskonomy when K=4}
    \label{}
\end{table*}

\begin{table*}[t]
\centering
\resizebox{0.99\textwidth}{!}{
    \begin{tabular}{l|l|ccccc}
    \hline
Method                   & Splits  & Depth estimation  & Surface normal    & Semantic segmentation & Keypoint detection & Canny edge detection \\ \hline
\multirow{5}{*}{HOA}     & group 1 & -                 & \checkmark          & -                     & \checkmark           & -                    \\
                         & group 2 & -                 & -                 & -                     & \textcolor{red}{\checkmark}  & \textcolor{red}{\checkmark}    \\
                         & group 3 & -                 & \textcolor{red}{\checkmark} & \textcolor{red}{\checkmark}     & -         & -           \\
                         & group 4 & \textcolor{red}{\checkmark} & \checkmark          & -                     & -         & -           \\
                         & group 5 & -                 & \checkmark          & -                     & -         & -           \\ \hline
\multirow{5}{*}{TAG}     & group 1 & \checkmark          & -                 & \checkmark              & -                  & -                    \\
                         & group 2 & \textcolor{red}{\checkmark} & \checkmark          & -                     & -                  & -                    \\
                         & group 3 & -                 & -                 & -                     & \textcolor{red}{\checkmark}  & \textcolor{red}{\checkmark}    \\
                         & group 4 & \checkmark          & \textcolor{red}{\checkmark} & \textcolor{red}{\checkmark}     & -         & -           \\
                         & group 5 & \checkmark          & \checkmark          & \checkmark              & \checkmark           &                      \\ \hline
\multirow{5}{*}{MTG-Net} & group 1 & \checkmark          & \textcolor{red}{\checkmark} & \textcolor{red}{\checkmark}     & \checkmark           & \checkmark             \\
                         & group 2 & \checkmark          & \checkmark          & -                     & \textcolor{red}{\checkmark}  & -                    \\
                         & group 3 & \textcolor{red}{\checkmark} & \checkmark          & -                     & -                  & \textcolor{red}{\checkmark}    \\
                         & group 4 & \checkmark          & \checkmark          & -                     & -                  & -                    \\
                         & group 5 & -                 & -                 & -                     & -                  & -                    \\ \hline
\multirow{5}{*}{Ours}    & group 1 & -         &                   &                       & \textcolor{red}{\checkmark}  & \textcolor{red}{}            \\
                         & group 2 & -        & -                 & -                     & -                  & \textcolor{red}{\checkmark}    \\
                         & group 3 & \textcolor{red}{\checkmark} & -        & -           & -          & -                    \\
                         & group 4 & -        & -                 & -                     & -                  & -           \\
                         & group 5 & -                 & \textcolor{red}{\checkmark} & \textcolor{red}{\checkmark}     & -                  & -                    \\ \hline                    
\end{tabular}}
    \caption{task loss on taskonomy when K=5}
    \label{}
\end{table*}

\begin{table*}[t]
\centering
\resizebox{0.99\textwidth}{!}{
    \begin{tabular}{l|l|cc|cc|cc|cc|cc|cc|cc|cc|cc}
    \hline
\multirow{2}{*}{Groups} & \multirow{2}{*}{Methods} & \multicolumn{2}{c|}{\makecell{5\_o\_Clock\_\\Shadow}} & \multicolumn{2}{c|}{\makecell{Black\_Hair}} & \multicolumn{2}{c|}{Blond\_Hair} & \multicolumn{2}{c|}{Brown\_Hair} & \multicolumn{2}{c|}{Goatee} & \multicolumn{2}{c|}{Mustache} & \multicolumn{2}{c|}{No\_Beard} & \multicolumn{2}{c|}{Rosy\_Cheeks} & \multicolumn{2}{c}{Wearing\_Hat} \\ \cline{3-20}
                        &                          & Error $\downarrow$             & \makecell[c]{Norm-\\Gain $\uparrow$}            & Error $\downarrow$         & \makecell[c]{Norm-\\Gain $\uparrow$}        & Error $\downarrow$         & \makecell[c]{Norm-\\Gain $\uparrow$}        & Error $\downarrow$         & \makecell[c]{Norm-\\Gain $\uparrow$}        & Error $\downarrow$      & \makecell[c]{Norm-\\Gain $\uparrow$}      & Error $\downarrow$       & \makecell[c]{Norm-\\Gain $\uparrow$}       & Error $\downarrow$        & \makecell[c]{Norm-\\Gain $\uparrow$}       & Error $\downarrow$         & \makecell[c]{Norm-\\Gain $\uparrow$}         & Error $\downarrow$         & \makecell[c]{Norm-\\Gain $\uparrow$}         \\ \hline
                        & MTL                      & 6.74              &-                     & 11.80         &-                 & 4.99          &-                 & 13.72         &-                 & 3.03       &-               & 3.71        &-                & 5.57         &-                & 5.20          &-                  & 1.36          &-                  \\
                        & STL                      & 7.60              & -12.78              & 13.30         & -12.69          & 5.46          & -9.33           & 12.46         & 9.16            & 3.47       & -14.57        & 3.76        & -1.35          & 5.80         & -4.14          & 6.65          & -27.81           & 1.42          & -4.80            \\ \hline
\multirow{3}{*}{K=2}    & HOA                      & 6.99              & -3.64               & \textcolor{blue}{11.83}         & \textcolor{blue}{-0.21}           & 4.64          & 7.12            & \textcolor{blue}{12.05}         & \textcolor{blue}{12.16}           & \textcolor{blue}{3.04}       & \textcolor{blue}{-0.33}         & \textbf{3.58}        & \textbf{3.38}           & \textcolor{blue}{4.91}         & \textcolor{blue}{11.78}          & \textbf{5.19}          & \textbf{0.29}             & 1.37          & -1.10            \\
                        & TAG                      & \textcolor{blue}{6.71}              & \textcolor{blue}{0.44}                & 11.88         & -0.68           & \textcolor{blue}{4.53}          & \textcolor{blue}{9.23}            & \textbf{11.90}         & \textbf{13.29}           & 3.06       & -1.16         & \textcolor{blue}{3.59}        & \textcolor{blue}{3.24}           & 5.22         & 6.21           & \textcolor{blue}{5.30}          & \textcolor{blue}{-1.83}            & \textcolor{blue}{1.21}          & \textcolor{blue}{10.70}            \\
                        & Ours                     & \textbf{6.64}      & \textbf{1.56}      & \textbf{11.57} & \textbf{1.95}  & \textbf{4.48}  & \textbf{10.23} & 12.13 & 11.61 & \textbf{2.98} & \textbf{1.49} & 3.68 & 0.81 & \textbf{4.85} & \textbf{12.95} & 5.51  & -5.87  & \textbf{1.13}  & \textbf{16.98}            \\ \hline
\multirow{3}{*}{K=3}    & HOA                      & \textcolor{blue}{6.64}              & \textcolor{blue}{1.49}                & \textbf{11.42}         & \textbf{3.23}            & \textbf{4.65}          & \textbf{6.92}            & \textcolor{blue}{12.85}         & \textcolor{blue}{6.35}            & 3.04       & -0.33         & 3.96        & -6.76          & \textbf{4.91}         & \textbf{11.78}          & \textcolor{blue}{5.40}          & \textcolor{blue}{-3.75}            & \textbf{1.17}          & \textbf{13.66}            \\
                        & TAG                      & 6.71              & 0.44                & \textbf{11.42}         & \textbf{3.23}            & 5.11          & -2.41           & \textcolor{blue}{12.85}         & \textcolor{blue}{6.35}            & \textbf{2.87}       & \textbf{5.13}          & \textbf{3.42}        & \textbf{7.84}           & 5.12         & 8.09           & 5.44          & -4.43            & 1.43          & -5.53            \\
                        & Ours                     & \textbf{6.58}      & \textbf{2.45}      & \textcolor{blue}{11.98} & \textcolor{blue}{-1.49} & \textcolor{blue}{4.86}  & \textcolor{blue}{2.61}  & \textbf{12.27} & \textbf{10.59} & \textcolor{blue}{2.98} & \textcolor{blue}{1.49} & \textcolor{blue}{3.49} & \textcolor{blue}{5.95} & \textcolor{blue}{5.02} & \textcolor{blue}{9.89}  & \textbf{5.31}  & \textbf{-1.93}  & \textcolor{blue}{1.19}  & \textcolor{blue}{12.18}            \\ \hline
\multirow{3}{*}{K=4}    & HOA                      & \textbf{6.69}              & \textbf{0.82}                & \textbf{11.42}         & \textbf{3.23}            & 5.11          & -2.41           & \textcolor{blue}{12.85}         & \textcolor{blue}{6.35}            & \textbf{2.87}       & \textbf{5.13}          & \textbf{3.42}        & \textbf{7.84}           & \textbf{4.91}         & \textbf{11.78}          & 5.44          & -4.43            & 1.43          & -5.53            \\
                        & TAG                      & \textcolor{blue}{6.71}              & \textcolor{blue}{0.44}                & \textbf{11.42}         & \textbf{3.23}            & \textcolor{blue}{4.77}          & \textcolor{blue}{4.41}            & \textcolor{blue}{12.85}         & \textcolor{blue}{6.35}            & \textcolor{blue}{2.96}       & \textcolor{blue}{2.15}          & 3.64        & 1.76           & 5.22         & 6.21           & \textbf{5.23}          & \textbf{-0.48}            & \textcolor{blue}{1.30}          & \textcolor{blue}{4.43}             \\
                        & Ours                     & 6.87      & -1.86     & \textcolor{blue}{11.53} & \textcolor{blue}{2.29}  & \textbf{4.65}  & \textbf{6.92}  & \textbf{12.37} & \textbf{9.86}  & 2.99 & 1.16 & \textcolor{blue}{3.50} &\textcolor{blue}{5.54} & \textcolor{blue}{5.12} & \textcolor{blue}{8.09}  & \textcolor{blue}{5.42}  & \textcolor{blue}{-4.04}  & \textbf{1.17}  & \textbf{13.66}           \\ \hline
\end{tabular}}
    \caption{celeb\_a. The first is marked as bold, while the second is blue.}
    \label{tab:celeb_a_per_task}
\end{table*}

\begin{table*}[t]
\centering
\resizebox{0.99\textwidth}{!}{
    \begin{tabular}{l|l|ccccccccc}
    \hline
Methods               & Splits  & 5\_o\_Clock\_Shadow & Black\_Hair & Blond\_Hair & Brown\_Hair & Goatee & Mustache & No\_Beard & Rosy\_Cheeks & Wearing\_Hat \\ \hline
\multirow{2}{*}{HOA}  & group 1 & \textcolor{red}{\checkmark}          & \textcolor{red}{\checkmark}  & \textcolor{red}{\checkmark}  & \textcolor{red}{\checkmark}  & -          & \textcolor{red}{\checkmark} & -          & \textcolor{red}{\checkmark}   & \textcolor{red}{\checkmark}   \\
                      & group 2 & -                   & -           & -           & -           & \textcolor{red}{\checkmark} & -          & \textcolor{red}{\checkmark} & -            & -            \\ \hline
\multirow{2}{*}{TAG}  & group 1 & \textcolor{red}{\checkmark}          & -           & -           & -           & -          & -          & \textcolor{red}{\checkmark} & -            & -            \\
                      & group 2 & -                   & \textcolor{red}{\checkmark}  & \textcolor{red}{\checkmark}  & \textcolor{red}{\checkmark}  & \textcolor{red}{\checkmark} & \textcolor{red}{\checkmark} & -          & \textcolor{red}{\checkmark}   & \textcolor{red}{\checkmark}   \\ \hline
\multirow{2}{*}{Ours} & group 1 & \textcolor{red}{\checkmark}                   & \textcolor{red}{\checkmark}           & -           & \textcolor{red}{\checkmark}           & -      & -        & -         & -            & \textcolor{red}{\checkmark}            \\
                      & group 2 & -                   & -           & \textcolor{red}{\checkmark}           & -           & \textcolor{red}{\checkmark}      & \textcolor{red}{\checkmark}        & \textcolor{red}{\checkmark}         & \textcolor{red}{\checkmark}            & -            \\     \hline              
\end{tabular}}
    \caption{celeb\_a when K=2}
    \label{}
\end{table*}

\begin{table*}[t]
\centering
\resizebox{0.99\textwidth}{!}{
    \begin{tabular}{l|l|ccccccccc}
    \hline
Methods               & Splits  & 5\_o\_Clock\_Shadow & Black\_Hair & Blond\_Hair & Brown\_Hair & Goatee & Mustache & No\_Beard & Rosy\_Cheeks & Wearing\_Hat \\ \hline
\multirow{3}{*}{HOA}  & group 1 & \textcolor{red}{\checkmark}          & -           & \textcolor{red}{\checkmark}  & -           & \textcolor{red}{\checkmark} & \textcolor{red}{\checkmark} & \checkmark          & \textcolor{red}{\checkmark}   & \textcolor{red}{\checkmark}   \\
                      & group 2 & -                   & \textcolor{red}{\checkmark}  & -           & \textcolor{red}{\checkmark}  & -          & -          & -          & -            & -            \\
                      & group 3 & -                   & -           & -           & -           & \checkmark          & -          & \textcolor{red}{\checkmark} & -            & -            \\ \hline
\multirow{3}{*}{TAG}  & group 1 & \textcolor{red}{\checkmark}          & -           & -           & -           & -          & -          & \checkmark          & -            & -            \\
                      & group 2 & -                   & \checkmark           & \textcolor{red}{\checkmark}  & -           & \textcolor{red}{\checkmark} & \textcolor{red}{\checkmark} & \textcolor{red}{\checkmark} & \textcolor{red}{\checkmark}   & \textcolor{red}{\checkmark}   \\
                      & group 3 & -                   & \textcolor{red}{\checkmark}  & -           & \textcolor{red}{\checkmark}  & -          & -          & -          & -            & -            \\ \hline
\multirow{3}{*}{Ours} & group 1 & \textcolor{red}{\checkmark}          & -           & -           & \textcolor{red}{\checkmark}  & \textcolor{red}{\checkmark} & -          & \textcolor{red}{\checkmark} & -            & \textcolor{red}{\checkmark}   \\
                      & group 2 & -                   & \textcolor{red}{\checkmark}  & -           & -           & -          & \textcolor{red}{\checkmark} & -          & -            & -            \\
                      & group 3 & -                   & -           & \textcolor{red}{\checkmark}  & -           & -          & -          & -          & \textcolor{red}{\checkmark}   & -            \\     \hline              
\end{tabular}}
    \caption{celeb\_a when K=3}
    \label{}
\end{table*}

\begin{table*}[t]
\centering
\resizebox{0.99\textwidth}{!}{
    \begin{tabular}{l|l|ccccccccc}
    \hline
Methods               & Splits  & 5\_o\_Clock\_Shadow & Black\_Hair & Blond\_Hair & Brown\_Hair & Goatee & Mustache & No\_Beard & Rosy\_Cheeks & Wearing\_Hat \\ \hline
\multirow{4}{*}{HOA}  & group 1 & \textcolor{red}{\checkmark}          & -           & -           & -           & \checkmark          & -          & -          & -            & -            \\
                      & group 2 & -                   & \checkmark           & \textcolor{red}{\checkmark}  & -           & \textcolor{red}{\checkmark} & \textcolor{red}{\checkmark} & \checkmark          & \textcolor{red}{\checkmark}   & \textcolor{red}{\checkmark}   \\
                      & group 3 & -                   & \textcolor{red}{\checkmark}  & -           & \textcolor{red}{\checkmark}  & -          & -          & -          & -            & -            \\
                      & group 4 & -                   & -           & -           & -           & \checkmark          & -          & \textcolor{red}{\checkmark} & -            & -            \\ \hline
\multirow{4}{*}{TAG}  & group 1 & \textcolor{red}{\checkmark}          & -           & -           & -           & -          & -          & \textcolor{red}{\checkmark} & -            & -            \\
                      & group 2 & -                   & \checkmark           & \textcolor{red}{\checkmark}  & \checkmark           & -          & -          & \checkmark          & \textcolor{red}{\checkmark}   & \textcolor{red}{\checkmark}   \\
                      & group 3 & -                   & \textcolor{red}{\checkmark}  & -           & \textcolor{red}{\checkmark}  & -          & -          & -          & -            & -            \\
                      & group 4 & -                   & -           & -           & -           & \textcolor{red}{\checkmark} & \textcolor{red}{\checkmark} & -          & -            & -            \\ \hline
\multirow{4}{*}{Ours} & group 1 & -                   & -           & -           & -           & -          & -          & -          & -            & \textcolor{red}{\checkmark}   \\
                      & group 2 & \textcolor{red}{\checkmark}          & -           & \textcolor{red}{\checkmark}  & -           & -          & \textcolor{red}{\checkmark} & -          & -            & -            \\
                      & group 3 & -                   & -           & -           & \textcolor{red}{\checkmark}  & -          & -          & -          & -            & -            \\
                      & group 4 & -                   & \textcolor{red}{\checkmark}  & -           & -           & \textcolor{red}{\checkmark} & -          & \textcolor{red}{\checkmark} & \textcolor{red}{\checkmark}   & - \\     \hline              
\end{tabular}}
    \caption{celeb\_a when K=4}
    \label{}
\end{table*}
%%%%%%%%%%%%%%%%%%%%%%%%%%%%%%%%%%%%%%%%%%%%%%%%%%%%%%%%%%%%%%%%%%%%%%%%%%%%%%%
%%%%%%%%%%%%%%%%%%%%%%%%%%%%%%%%%%%%%%%%%%%%%%%%%%%%%%%%%%%%%%%%%%%%%%%%%%%%%%%
